# Supplementary material for: Inference on Local Average Treatment Effects for Misclassified Treatment
Source: arXiv:1804.03349 ancillary file (2018-04-10)
Supplement: Supplementary file 1 [file supplement.pdf]

# Supplementary Appendix of "Inference on Local Average Treatment Effects for Misclassified Treatment"

Takahide Yanagi*

April 10, 2018

This supplementary file contains additional results that are omitted from the main body of the paper. Appendix B examines a measurement error for the outcome $Y$ or the instrument $Z$. Appendix C develops identification when the instrument $Z$ is multi-valued. Appendix D gives the necessary and sufficient conditions of the inequalities in Assumption 4.4. Appendix E discusses the interpretation of the identified parameters when the roles of binary instruments $Z$ and $V$ are changed.

## B Appendix: Mismeasured outcome or instrument

This appendix considers the situation in Remark 1 in which $Y \in \mathbb{R}$ or $Z \in \{0,1\}$ may be a mismeasured variable of the true unobserved variable $Y^* \in \mathbb{R}$ or $Z^* \in \{0,1\}$, respectively. Here, we assume that treatment $T = T^*$ is observed without a measurement error for simplicity.

We first consider that continuous outcome $Y$ may be a mismeasured variable of true continuous $Y^*$. By assuming that measurement error $U_Y := Y - Y^*$ satisfies $E(U_Y|Z =$

*Graduate School of Economics, Hitotsubashi University, 2-1 Naka, Kunitachi, Tokyo 186-8601, Japan. Email: t.yanagi@r.hit-u.ac.jp

$1) = E(U_Y|Z = 0)$, it holds that

$$\frac{E(Y|Z = 1) - E(Y|Z = 0)}{E(T|Z = 1) - E(T|Z = 0)} = \frac{E(Y^*|Z = 1) - E(Y^*|Z = 0)}{E(T|Z = 1) - E(T|Z = 0)}.$$

Thus, the observable IV estimand identifies the LATE, meaning that the measurement error that is mean-independent of the instrument does not contaminate the inference.

We note that the measurement error for discrete $Y$ may not satisfy the condition of $E(U_Y|Z = 1) = E(U_Y|Z = 0)$ as in the analysis of the mismeasured binary treatment in this study. The measurement error for the discrete outcome should be analyzed based on other approaches.

We then consider the situation under which $Z$ may be a misclassified variable of true $Z^*$. The true parameter and observable analogue are

$$\frac{E(Y|Z^* = 1) - E(Y|Z^* = 0)}{E(T|Z^* = 1) - E(T|Z^* = 0)}, \quad \text{and} \quad \frac{E(Y|Z = 1) - E(Y|Z = 0)}{E(T|Z = 1) - E(T|Z = 0)},$$

respectively. Note that for each $z = 0, 1$, $E(Y|Z = z) = E(Y|Z^* = 1 - z)\Pr(Z^* = 1 - z|Z = z) + E(Y|Z^* = z)\Pr(Z^* = z|Z = z)$ under the non-differential measurement error $E(Y|Z^*, Z) = E(Y|Z^*)$. Hence, we have $E(Y|Z = 1) - E(Y|Z = 0) = [E(Y|Z^* = 1) - E(Y|Z^* = 0)][\Pr(Z^* = 1|Z = 1) - \Pr(Z^* = 1|Z = 0)]$. By using the same procedure, we can show that $E(T|Z = 1) - E(T|Z = 0) = [E(T|Z^* = 1) - E(T|Z^* = 0)][\Pr(Z^* = 1|Z = 1) - \Pr(Z^* = 1|Z = 0)]$ under the non-differential measurement error $E(T|Z^*, Z) = E(T|Z^*)$. Therefore, we have

$$\frac{E(Y|Z = 1) - E(Y|Z = 0)}{E(T|Z = 1) - E(T|Z = 0)} = \frac{E(Y|Z^* = 1) - E(Y|Z^* = 0)}{E(T|Z^* = 1) - E(T|Z^* = 0)}.$$

Thus, the non-differential measurement error for $Z$ does not contaminate the inference.

# C Appendix: Inference with a multi-valued instrument

As discussed in Remark 2, the identification and GMM inference proposed in the main body can be extended to the setting where a binary treatment may be misclassified and an instrument is multi-valued discrete (i.e., non-binary). Without measurement errors, Imbens and Angrist (1994) develop the identification of a LATE with a discrete instrument. Let $Y \in \mathbb{R}$ be the outcome, $T \in \{0,1\}$ be the possibly misclassified binary treatment for the true treatment $T^* \in \{0,1\}$, and $Z \in \{z_1, z_2, \ldots, z_L\}$ be the multi-valued discrete instrument. The true and observable IV estimands are

$$\beta^* = \frac{Cov(Y,Z)}{Cov(T^*,Z)}, \qquad \beta = \frac{Cov(Y,Z)}{Cov(T,Z)}, \tag{20}$$

respectively. Under identification conditions, Imbens and Angrist (1994, Section 3) show that $\beta^*$ identifies a weighted average of the LATEs $E[Y_1 - Y_0 | T^*_{z_{l+1}} = 1, T^*_{z_l} = 0]$, where $T^*_{z_l}$ is the potential treatment when $Z = z_l$ for $l = 1, 2, \ldots, L-1$.

When observed $T$ contains a measurement error, the problem of identifying $\beta^*$ is that $\beta$ is not generally equal to $\beta^*$. Because the numerators of $\beta^*$ and $\beta$ are identical, we focus on the denominators. Recalling the shorthand notations $p^*_z = \Pr(T^* = 1|Z = z)$, $p_z = \Pr(T = 1|Z = z)$, and $r = E(Z)$, it is easy to see that

$$Cov(T^*,Z) = \sum_{l=1}^{L} p^*_{z_l} z_l \Pr(Z = z_l) - r \sum_{l=1}^{L} p^*_{z_l} \Pr(Z = z_l), \tag{21}$$

and

$$Cov(T,Z) = \sum_{l=1}^{L} p_{z_l} z_l \Pr(Z = z_l) - r \sum_{l=1}^{L} p_{z_l} \Pr(Z = z_l),$$

according to the law of iterated expectations. It also holds that

$$p^*_{z_l} = \frac{p_{z_l} - m_{0z_l}}{s_{z_l}},$$

as shown in (5), where $m_{tz_l} = \Pr(T \neq T^*|T^* = t, Z = z_l)$ and $s_{z_l} = 1 - m_{0z_l} - m_{1z_l}$. These observations imply that $p^*_{z_l} \neq p_{z_l}$ in general, so that $\beta$ does not identify $\beta^*$ in general.

When we observe an exogenous variable $V$, we can identify $\beta^*$ by carrying out almost the same procedure as in Section 4. If we assume the existence of at least three-valued discrete exogenous $V \in \{v_1, v_2, \ldots, v_K\}$ with Assumptions 4.1, 4.2, 4.3, and 4.4 (i) for $z = z_1, z_2, \ldots, z_L$, then $\beta^*$ is identified based on (20) and (21) since $p^*_{z_l}$ and $m_{tz_l}$ are identified based on the same procedure in the discussion after Theorem 1. Further, if we additionally assume $m_{tz_l} = m_t$ as in Assumption 4.4 (ii), $V$ can be binary for the identification.

The GMM inference may be conducted based on the moment conditions implied by the identification. We first explain the moment conditions for non-binary $V \in \{v_1, v_2, \ldots, v_K\}$. Defining the shorthand notation $\sigma_{T^*Z} := Cov(T^*, Z)$, suppose that the vector of the true parameters is

$$\theta_0 = \Big(\beta^*, \sigma_{T^*Z}, r, \big\{(m_{0z_l}, m_{1z_l}, \{p^*_{vz_l}\}_{v=v_1}^{v_K}, \tau_{z_l})\big\}_{l=1}^{L}\Big)^\top,$$

which contains $L(K+3)+3$ elements. The moment conditions implied by the identification are $E[g(X, \theta_0)] = 0$, where $X = (Y, T, Z, V)^\top$ and the vector-valued function $g(X, \theta_0)$ is composed of the following $2LK + 3$ elements.

$$\begin{aligned}
& r - Z, \\
& \Big(m_{0z} + (1 - m_{0z} - m_{1z})p^*_{zv_k} - T\Big) I_{zv_k}, \\
& \left(\tau^*_z + \frac{YT - (1 - m_{1z})p^*_{zv_k}\tau^*_z}{m_{0z} + (1 - m_{0z} - m_{1z})p^*_{zv_k}} - \frac{Y(1-T) + (1 - m_{0z})(1 - p^*_{zv_k})\tau^*_z}{1 - (m_{0z} + (1 - m_{0z} - m_{1z})p^*_{zv_k})}\right) I_{zv_k}, \\
& \sigma_{T^*Z} - \left(\sum_{l=1}^{L}\sum_{k=1}^{K} p^*_{z_lv_k} z_l I_{z_lv_k} - r\sum_{l=1}^{L}\sum_{k=1}^{K} p^*_{z_lv_k} I_{z_lv_k}\right), \\
& \beta^* - \frac{YZ - Yr}{\sigma_{T^*Z}},
\end{aligned}$$

where $I_{zv_k} = \mathbf{1}(Z = z, V = v_k)$ is the indicator. The first three elements are the same as those in (11). The last two elements are implied by the first equation in (20) and the

following equality similar to (21).

$$Cov(T^*, Z) = \sum_{l=1}^{L}\sum_{k=1}^{K} p^*_{z_l v_k} z_l \Pr(Z = z_l, V = v_k) - r\sum_{l=1}^{L}\sum_{k=1}^{K} p^*_{z_l v_k} \Pr(Z = z_l, V = v_k).$$

The number of overidentification restrictions is $L(K-3)$ and $\theta_0$ is just-identified when $V$ takes three values. Based on the moment conditions, we can consistently estimate $\theta_0$ by using the GMM estimation, as discussed in Remark 8.

The moment conditions above can be extended to the situation where $V \in \{v_1, v_2\}$ is binary. In this case, we have to assume $m_{tz_l} = m_t$ for $t = 0, 1$ and $l = 1, 2, \ldots, L$ additionally. Under the assumption of $m_{tz_l} = m_t$, we have the following vector of the $3L + 5$ parameters to be estimated:

$$\theta_0 = \left(\beta^*, \sigma_{T^*Z}, r, m_0, m_1, \{(p^*_{v_1 z_l}, p^*_{v_2 z_l}, \tau_{z_l})\}_{l=1}^{L}\right)^\top,$$

and the vector of the $4L+3$ moment conditions as in (20), implying $L-2$ overidentifying restrictions. Hence, $\theta_0$ is identified even with binary $V$, and the number of overidentifying restrictions depends on the number of elements in support of $Z$.

# D Appendix: Necessary and sufficient conditions of the inequalities in Assumption 4.4

This appendix presents the necessary and sufficient conditions of the inequalities in Assumptions 4.4 (i) and (ii). To this end, we first note that (12) and (13) lead to

$$\tau_W = \left(\frac{(1-m_1)p^*_W}{p_W} - \frac{m_1 p^*_W}{1-p_W}\right)\tau^*_Z \quad \Longleftrightarrow \quad \tau_W = \frac{p^*_W(1-m_1-p_W)}{p_W(1-p_W)}\tau^*_Z,$$

under Assumption 4.3. Here, from (15), we have $1-p^*_W = (1-m_{1Z}-p_W)/(1-m_{0Z}-m_{1Z})$. It thus holds that

$$\tau_W = \frac{p^*_W(1-p^*_W)}{p_W(1-p_W)}(1-m_{0Z}-m_{1Z})\tau^*_Z. \tag{22}$$

By defining $R_W := p_W^*(1-p_W^*)/[p_W(1-p_W)]$, we have $\tau_W = R_W(1-m_{0Z}-m_{1Z})\tau_Z^*$.

We next show that Assumption 4.4 (i) is identical to $\tau_z^* \neq 0$ and $m_{0z}+m_{1z} \neq 1$ for each $z = 0, 1$. According to (22), the equation in the assumption is rearranged as

$$\begin{aligned}
&\left(\frac{\tau_{zv_1}}{p_{zv_2}} - \frac{\tau_{zv_2}}{p_{zv_1}}\right)\left(\frac{\tau_{zv_1}}{1-p_{zv_3}} - \frac{\tau_{zv_3}}{1-p_{zv_1}}\right) - \left(\frac{\tau_{zv_1}}{1-p_{zv_2}} - \frac{\tau_{zv_2}}{1-p_{zv_1}}\right)\left(\frac{\tau_{zv_1}}{p_{zv_3}} - \frac{\tau_{zv_3}}{p_{zv_1}}\right) \\
&= \left[\left(\frac{R_{zv_1}}{p_{zv_2}} - \frac{R_{zv_2}}{p_{zv_1}}\right)\left(\frac{R_{zv_1}}{1-p_{zv_3}} - \frac{R_{zv_3}}{1-p_{zv_1}}\right) - \left(\frac{R_{zv_1}}{1-p_{zv_2}} - \frac{R_{zv_2}}{1-p_{zv_1}}\right)\left(\frac{R_{zv_1}}{p_{zv_3}} - \frac{R_{zv_3}}{p_{zv_1}}\right)\right] \\
&\quad \times (1-m_{0z}-m_{1z})\tau_z^*.
\end{aligned}$$

Therefore, under Assumption 4.3, the inequality in Assumption 4.1 (i) is satisfied if and only if $m_{0z}+m_{1z} \neq 1$ and $\tau_z^* \neq 0$ for each $z = 0, 1$.

We next show that the necessary and sufficient condition of the inequality in Assumption 4.4 (ii) is also that $m_{0z}+m_{1z} \neq 1$ and $\tau_z^* \neq 0$ for each $z = 0, 1$. Under the condition that $m_0 = m_{00} = m_{01}$ and $m_1 = m_{10} = m_{11}$, the equation in the assumption is rewritten as

$$\begin{aligned}
&\left(\frac{\tau_{0v_1}}{p_{0v_2}} - \frac{\tau_{0v_2}}{p_{0v_1}}\right)\left(\frac{\tau_{1v_1}}{1-p_{1v_2}} - \frac{\tau_{1v_2}}{1-p_{1v_1}}\right) - \left(\frac{\tau_{0v_1}}{1-p_{0v_2}} - \frac{\tau_{0v_2}}{1-p_{0v_1}}\right)\left(\frac{\tau_{1v_1}}{p_{1v_2}} - \frac{\tau_{1v_2}}{p_{1v_1}}\right) \\
&= \left(\frac{R_{0v_1}}{p_{0v_2}} - \frac{R_{0v_2}}{p_{0v_1}}\right)\left(\frac{R_{1v_0}}{1-p_{1v_2}} - \frac{R_{1v_2}}{1-p_{1v_1}}\right) - \left(\frac{R_{0v_1}}{1-p_{0v_2}} - \frac{R_{0v_2}}{1-p_{0v_1}}\right)\left(\frac{R_{1v_1}}{p_{1v_2}} - \frac{R_{1v_2}}{p_{1v_1}}\right) \\
&\quad \times (1-m_0-m_1)\tau_0^*\tau_1^*,
\end{aligned}$$

where we use (22). Hence, under Assumption 4.3, the inequality in Assumption 4.4 (ii) is satisfied if and only if $\tau_z^* \neq 0$ and $m_0+m_1 \neq 1$ for each $z = 0, 1$.

# E Appendix: Interpretation of the roles of binary $Z$ and $V$

As discussed in Remark 6, when $V$ is a binary instrument as well as $Z$, we can consider the analysis in which the roles of $Z$ and $V$ are changed. To see this, suppose that $\tilde{T}_0^*$ and $\tilde{T}_1^*$ are the potential true treatment statuses when $V = 0$ and $V = 1$, respectively. Then,

the LATE based on the instrument $V$ is

$$E(Y_1 - Y_0 | \tilde{T}_1^* > \tilde{T}_0^*), \tag{23}$$

which is the average causal effect for compliers whose treatment statuses are positively altered with the value of $V$. Under Assumptions 3.1, 3.2, and 3.3 with $V$ in place of $Z$, the LATE in (23) satisfies the following equation:

$$E(Y_1 - Y_0 | \tilde{T}_1 > \tilde{T}_0) = \frac{E(Y|V=1) - E(Y|V=0)}{E(T^*|V=1) - E(T^*|V=0)}.$$

Further, if Assumptions 4.1, 4.2, 4.3, and 4.4 are satisfied with $Z$ and $V$ in place of $V$ and $Z$, respectively, the LATE and misclassification probabilities are identified by adopting the same procedure as in the main body.

In practice, both LATEs in (1) and (23) may be identified based on the information on $(Y, T, Z, V)$; however, the LATE in (23) might be different from the LATE in (1) since the definition of compliers might depend on which of $Z$ and $V$ is the instrument. For example, when we select using one of the two indicators of two-year and four-year college proximity as $Z$, compliers based on two-year college proximity (i.e., individuals graduate if and only if they live close to two-year colleges) might be different from those based on four-year college proximity (i.e., individuals graduate if and only if they live close to four-year colleges). As a result, the LATE based on two-year college proximity might be different from that based on four-year college proximity. In such a case, which of the LATEs in (1) and (23) should be the main parameter of interest would depend on the situation of the empirical application. Specifically, the main parameter of interest should be determined by assessing which of the compliers based on $Z$ and $V$ is of more interest or by comparing the magnitudes of the first-stage regressions. Of course, if the members of the compliers do not depend on changing the roles of $Z$ and $V$, both the LATEs in (1) and (23) are identical and identified.

# References

G. W. Imbens and J. D. Angrist. Identification and estimation of local average treatment effects. *Econometrica*, 62(2):467–475, 1994.
